# Supplementary material for: Onset of turbulence in channel flows with scale-invariant roughness
Source: arXiv:2006.16169 source file (2020-06-29)
Supplement: Supplementary file 1 [file supplement.pdf]

# Supplemental Material: Onset of turbulence in channel flows with scale-invariant roughness


Gaute Linga,[1,2] Luiza Angheluta,[1] and Joachim Mathiesen[2]

[1] *PoreLab, The Njord Center, Department of Physics, University of Oslo, P.O. Box 1048, Blindern, N-0316 Oslo, Norway*

[2] *Niels Bohr Institute, University of Copenhagen, Blegdamsvej 17, DK-2100 Copenhagen, Denmark*



(Dated: June 27, 2020)



This supplemental material provides details about flow geometry, mesh generation, numerical simulations and the simulation protocol used. Additionally, we provide some basic observations of the aperture and velocity fields which may facilitate reproducibility.


## I. FRACTURE GEOMETRY AND MESH

In this section we describe the geometry of the rough channels, and the computational meshes used to represent them.

### A. Self-affine channel

There is significant evidence for fracture surfaces being self-affine [1]. We therefore choose to study a system comprised of two identical, vertically shifted (along $z$), self-affine surfaces $z = h(x, y)$ and $z = h(x, y) + d$. Together they form a channel of constant height $d$, wherein an incompressible fluid is forced to flow along the $x$ axis. This direction is henceforth called the streamwise direction, while the $y$ direction is called the spanwise direction. In geoscience, this type of geometry is known as a fracture joint, resulting from mode I fracture, in contrast to a fault, where the surfaces would be shifted both vertically and in the $xy$ plane [2].

The self-affine profile is described as a 2D surface in 3D space, which is statistically invariant under the transformation

$$x \to \lambda x, \quad y \to \lambda y, \quad z \to \lambda^H z. \tag{1}$$

Using a self-affine surface is also a simple and generic way of describing a rough surface profile where as few as possible length scales are involved. In addition to the Hurst exponent $H$, there needs to be specified a lower cut-off (larger than the finite element size $\Delta x$), and a system size, $L$. However, this does not fully fix the vertical undulation of the surface. We therefore specify a root-mean-square height deviation, $A = L^{-1}\sqrt{\int_0^L \int_0^L h^2(x, y)\,\mathrm{d}x\,\mathrm{d}y}$, which we call *roughness amplitude*, which ultimately fixes the surface. Clearly, due to the self-affine nature of the surface, the latter scales with the finite system size as $A \sim L^H$. It is therefore evident that a proper study of the scaling properties of flow in self affine geometries would require to properly correct for finite-size effects, etc., which has been done in the lubrication approximation (see e.g. [3]), but is computationally costly for DNS in 3D. With this in mind, we will in the present work hold $L$ fixed, leaving a scaling analysis for future work.

Our motivation for using a self-affine channel is twofold: (i) It is a simple way to introduce a random perturbation to an otherwise linearly stable flow, and (ii) it is a physically relevant system as it results from natural processes, such as brittle fractures [1, 4] and surface growth [5].

### B. Computational meshes

Unstructured tetrahedral meshes are generated by first constructing a $256 \times 256$ (lattice units) self-affine surface with $H = 0.8$ using a Fourier filtering method [6]. There are several other ways of constructing such surfaces, but the Fourier method has the advantage that it results in a periodic surface, which will be of importance in imposing periodic boundary conditions on the flow field. To check that the surface is actually self-affine with the correct Hurst exponent, we compare the power spectrum of the surface height (measured along a line in the plane) with the theoretical one,

$$P(k_i) \sim k_i^{-1-2H}, \quad \text{for} \quad i \in \{x, y\}, \tag{2a}$$

$$P(k_r) \sim k_r^{-1-H}. \tag{2b}$$

Here, $\mathbf{k} = (k_x, k_y)$ is the wave vector in Fourier space and $k_r = |\mathbf{k}|$. The power spectrum of the self-affine surface is shown in Fig. 1, and is seen to yield a self-affine scaling, consistent with (2), over roughly two orders of magnitude.

After the self-affinity has been established, we interpolate the surface smoothly (using bicubic interpolation) between all the points of the lattice, in order to remove sharp edges in the mesh that could cause unsought numerical inaccuracies. Note that this implies that the roughness cut-off scale is somewhat larger than the mesh size. The resulting $512 \times 512\Delta x^2$ surface, which is ensured to be periodic, is scaled in the plane to $10 \times 10$ simulation units. The surface height is rescaled to yield a specified roughness amplitude $A$. The surface mesh is then copied and shifted a distance $d$ vertically. At the corners making up the slab, nodes are added with a spacing $\Delta x$. The side faces nodes are then triangulated (with a typical length $\Delta x$) using the MeshPy [7] interface to Triangle [8]. Finally, the interior of the slab is meshed using TetGen [9]. The mesh is refined near the surface

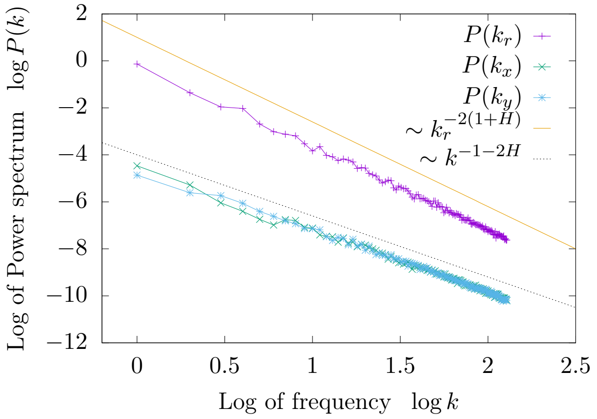


FIG. 1. Power spectrum of the self-affine surface used in this study, along $x$ and $y$ in Fourier space $(k_x, k_y)$, and radially averaged, $k_r$. The solid lines show the theoretical power spectra of a surface with the Hurst exponent $H = 0.8$.

to represent the complex surface (but to resolve turbulent flow, a fine mesh in the bulk is also necessary).

To address the effects of inertia and roughness, we have in the simulations used one single initial self-affine surface, with the power spectrum shown in Fig. 1. The roughness amplitudes have been chosen to be $A = 0, 0.1d, 0.2d, 0.5d$, and $0.8d$, as compared to the channel width $d = 1$. The four meshes used in this study are visualized in Fig. 2.

The properties of the surface meshes used in this study are listed in Table I. As is seen from the table, the surface area increases with the roughness amplitude $A$, but this is independent of the self-affine property, as any undulated surface should scale as $S^2(A) - S^2(0) \sim A^2$. Here, $S$ is the area of the self-affine part of the mesh with a given roughness scaling $A$, i.e. when the slab's faces are excluded. As a check, we verified that our meshes satisfy this. In principle, since $S \sim \Delta x^{-H}$, it is not expected to be finite for any nonzero roughness amplitude $A$. The surface that is *accessible* to the flow field will in any case be limited by the viscous boundary layer, which in the Reynolds number range we are considering is larger than this smallest scale.

TABLE I. Surface mesh information. The faces of the slabs are included.

| $A$ | Nodes | Facets | Total area | $\ell_{\text{facet}}$ |
|---|---|---|---|---|
| 0.0 | 698,146 | 1,396,288 | 240.0000 | 0.01311 |
| 0.1 | 698,606 | 1,397,208 | 245.4747 | 0.01325 |
| 0.2 | 699,008 | 1,398,012 | 260.5035 | 0.01365 |
| 0.5 | 698,382 | 1,396,760 | 339.2817 | 0.01558 |
| 0.8 | 697,110 | 1,394,216 | 441.2603 | 0.01779 |

The properties of the full mesh are listed in Table II. The number of nodes and elements in the meshes are fairly constant, as the meshes were generated using identical procedures.

TABLE II. Full mesh information, including bulk and surface.

| $A$ | Nodes | Elements | Volume | $\ell_{\text{elem}}$ |
|---|---|---|---|---|
| 0.0 | 3,696,368 | 21,526,314 | 100.0 | 0.0166 |
| 0.1 | 3,690,237 | 21,440,983 | 100.0 | 0.0167 |
| 0.2 | 3,672,117 | 21,302,242 | 100.0 | 0.0167 |
| 0.5 | 3,607,372 | 20,905,569 | 100.0 | 0.0168 |
| 0.8 | 3,518,454 | 20,382,889 | 100.0 | 0.0170 |

### C. Brief discussion of length scales

For transitional flow, Re $\sim$ 1000, the Kolmogorov scale $\ell_K$ is comparable to the typical element size $\ell_{\text{elem}}$ (cf. Table II), which is generally smaller than the most dissipative eddies. As a comparison, extrapolation of the relationship $\ell_K \sim \text{Re}^{-0.78}$ from the simulations by Mortensen and Valen-Sendstad [10] at a shear Reynolds number $\text{Re}_\tau \simeq 180$ (Re $\simeq$ 3000), yields a comparable grid scale. Since their simulations were almost indistinguishable from the reference data by Moser *et al.* [11], we estimate that our simulation results, which are mostly concerned with Re $\lesssim$ 2000, should be sufficiently well-resolved. (However, rough meshes at Re $\simeq$ 3000 will be pushing the limits.) This is particularly true as the dominating source of error lies, in our case, in the particular realization of a self-affine surface. Finally, we verified *a posteriori* that mesh refinement gave no significant change in the macroscopic flow properties even for the highest roughness.

## II. FLOW PROBLEM SETUP AND NUMERICAL METHOD

### A. Governing equations and problem setup

As outlined above, the setup we consider is a flow in a rough channel. We consider the domain $\Omega$ to be periodic in the $x$ and $y$ directions, and constrained by the same, shifted, rough surface above and below in the $z$ direction. The mean sampled over the $xy$ plane of the lower surface is at $z = 0$, and the mean at the upper surface is at $z = d$.

Within the slab, we perform direct numerical simulation (DNS) of fluid flow. The incompressible flow is governed by the Navier–Stokes equations:

$$\partial_t \mathbf{u} + \mathbf{u} \cdot \boldsymbol{\nabla} \mathbf{u} - \nu \boldsymbol{\nabla}^2 \mathbf{u} = -\boldsymbol{\nabla} p + \mathbf{f}, \quad \boldsymbol{\nabla} \cdot \mathbf{u} = 0. \tag{3}$$

Here $\mathbf{u}$ is the velocity field, $\nu$ is the kinematic viscosity, and $p$ is the pressure. For convenience of notation, we have absorbed the constant density into the latter quantity.

The flow is driven by a constant, uniform body force $\mathbf{f}$, either to a laminar or a transitionally turbulent flow

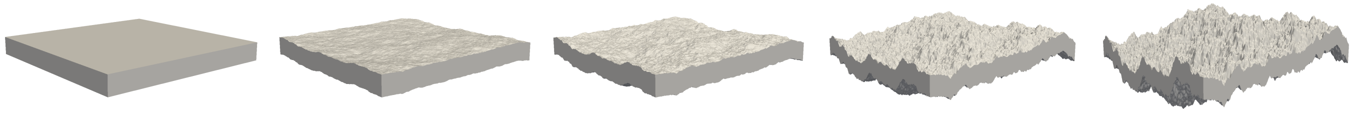

(a) $A = 0$ (b) $A = 0.1$ (c) $A = 0.2$ (d) $A = 0.5$ (e) $A = 0.8$

FIG. 2. The five meshes used in this study.

depending on the magnitude of $\mathbf{f}$. The force $\mathbf{f}$ is in the steady state (where the velocity is *at*, or temporally fluctuating around, a constant value) compensated by the friction between the flow field and the rough walls. At the same time it controls the injected energy per time, $\int_\Omega \mathbf{f}\cdot\mathbf{u}\,\mathrm{d}V$ ($V$ is volume), which is compensated by the (turbulent or laminar) dissipation rate, both at the walls and in the bulk. The present work is concerned with the transport properties of rough channels in this *statistical* steady state. The proper quantification of the transient dynamics of the transition process is left for future work.

In all simulations, no-slip conditions are applied at the boundaries, $\mathbf{u} = \mathbf{0}$ for $\mathbf{x} \in \partial\Omega$. In order not to trigger any spurious long-lived turbulent modes, we start all simulations from below, i.e. either at $\mathrm{Re} = 0$ or from a steady laminar or a transitional state below the sought Re.

### B. Numerical method

The finite element method (FEM) for fluid flow simulations in *regular* geometries such as smooth pipes, ducts, and channels, is usually outperformed by spectral methods. However, when complex boundaries are present, the latter methods cannot be applied without loss of performance. Irregular geometries, such as in our case of rough cracks, are accurately represented by unstructured meshes, which leaves the FEM as a viable option.

In order to numerically resolve the Navier–Stokes equations (3), we use a customized version of the Oasis software [10], which is both fast and highly flexible. Oasis is built on top of the FEniCS/Dolfin framework [12, 13], which in turn interfaces to highly optimized linear solvers through the PETSc backend [14]. In fact, although most of the user interaction with Oasis/FEniCS is through the high-level Python interface, the runtime of the simulations are dominated by the backend PETSc Krylov solvers. This makes the runtime comparable to e.g. OpenFOAM [15].

To discretize the flow equations, we use a temporally second-order incremental pressure correction scheme (IPCS) [10]. The equations we solve, at time $t = n\Delta t$ ($n$ is time step number, $\Delta t$ is the time step size), are

$$\frac{\mathbf{u}^* - \mathbf{u}^{n-1}}{\Delta t} + \hat{\mathbf{u}}\cdot\boldsymbol{\nabla}\tilde{\mathbf{u}} = \nu\boldsymbol{\nabla}^2\tilde{\mathbf{u}} - \boldsymbol{\nabla}p^* + \mathbf{f}, \tag{4a}$$

$$\boldsymbol{\nabla}^2\phi = -\frac{1}{\Delta t}\boldsymbol{\nabla}\cdot\mathbf{u}^*, \tag{4b}$$

$$\frac{\mathbf{u}^n - \mathbf{u}^*}{\Delta t} = -\boldsymbol{\nabla}\phi. \tag{4c}$$

Here, $\hat{\mathbf{u}} = (3\mathbf{u}^{n-1} - \mathbf{u}^{n-2})/2$ is an Adams–Bashforth projected advecting velocity, $\tilde{\mathbf{u}} = (\mathbf{u}^* + \mathbf{u}^{n-1})/2$ is the Crank–Nicholson interpolated advected velocity, and $\phi = p^{n-1/2} - p^*$ is an incremental pressure difference. In the above, velocity and pressure are solved in a segregated manner; Eq. (4a) is a velocity prediction step, Eq. (4b) is a pressure correction step, and Eq. (4c) is a velocity correction step. In this scheme, which is further documented in Ref. [10], Eqs. (4a) and (4b) are solved iteratively in an inner loop until a convergence criterion is reached, before in the end of a timestep (outer loop), Eq. (4c) is solved. For the spatial discretization, we use piecewise-linear Lagrange elements both for velocity and pressure ($\mathrm{P}_1$–$\mathrm{P}_1$), which yields second-order convergence in space.

### C. Simulation protocol

Figure 3 (a) shows an instantaneous snapshot of the velocity field in the statistical steady state. Here, it can be seen that transient flow patterns are present, particularly at the streamwise periodic cross-sectional plane, shown to the left in the figure.

To investigate the flow rate in time, we define a flux-based Reynolds number [16],

$$\mathrm{Re} = \frac{Q_x}{L\nu} = \frac{\langle u_x\rangle\, d}{\nu} \tag{5}$$

where $Q_x$ is the flux, i.e. volume per time, that passes through any (due to the incompressibility) cross section normal to the $x$-axis. Correspondingly, $\langle u_x\rangle$ is the mean velocity in the $x$ direction. We can interpret Eq. (5) either in an instantaneous or a in statistical sense, depending on whether $Q_x$ is a fluctuating quantity—which again will depend on the forcing $f$. In particular, for a given $f$, the *instantaneous Reynolds number* (for which we emphasize the time dependence by a subscript $t$) yields a unique value of Re in the following sense:

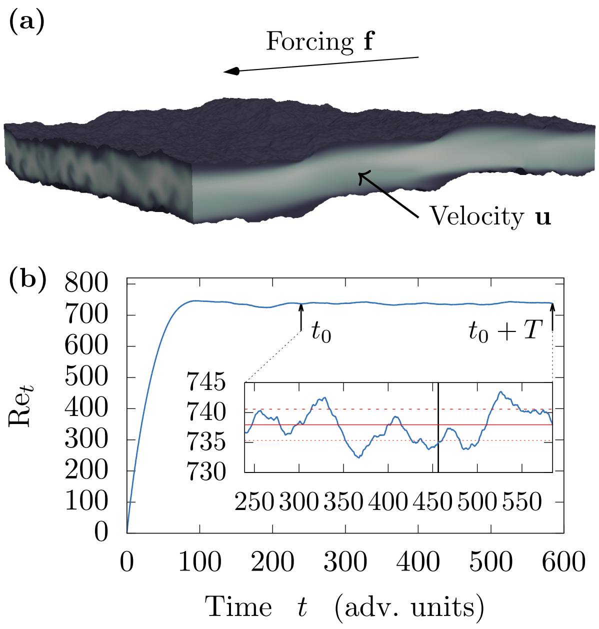


FIG. 3. A typical simulation in a self-affine channel with roughness amplitude $A = 0.2$, forcing $f = 1.5 \times 10^{-6}$ and viscosity $\nu = 9 \times 10^{-5}$. (a) A snapshot from the simulation after roughly 450 advective time units. The direction of forcing is shown, and the lighter color indicates higher speed. (b) Instantaneous Reynolds number $\mathrm{Re}_t$ (based on instantaneous flux) as a function of time. The time when a statistical steady state has been reached is indicated by $t_0$, and we indicate a sampling time $T$ over which statistical quantities are estimated. Inset: Amplification of the $\mathrm{Re}_t$ signal during the sampling time, and the eventually estimated Re is indicated by a horizontal solid red line. The standard deviation (shown around Re as horizontal dashed red lines) shows that the error in the time signal is less than 0.4%. The snapshot in (a) is taken at the time indicated by a vertical black line.

- If the flow is unsteady, Re is found as the average over a sufficiently long time in the statistical steady state, i.e. $\mathrm{Re} = \overline{\mathrm{Re}_t}$; or
- if the flow is laminar and steady, the relation is $\mathrm{Re} = \lim_{t\to\infty} \mathrm{Re}_t$.

The notion of the statistical steady state is exemplified in Fig. 3 (b). The latter shows the time evolution of $\mathrm{Re}_t$, in the simulation shown in Fig. 3 (a), starting from a quiescent state at $\mathrm{Re}_t = 0$. After an initial transient of exponential relaxation toward a steady value, a fluctuating signal develops. Indicated in the figure is a sampling interval between $t = t_0$, where the statistical steady state has been reached, and $t = t_0 + T$. The inset of Fig. 3 (b) shows a close-up of the velocity signal in the sampling interval, displaying a fluctuating behaviour. However, the standard deviation of this signal is less than 0.4% of Re, which is much less than the local fluctuations, meaning that $\lim_{t\to\infty} \mathrm{Re}_t \simeq \overline{\mathrm{Re}}$, and the steady and unsteady methods of computing Re are virtually equivalent.

For the case of high inertia (Re $\sim$ 1400), the velocity fields are well above the turbulent thresholds and thus strongly fluctuating in both time and space. In order to isolate the spatial fluctuations and visualize the mean transport channels, we therefore consider the *time-averaged velocity fields*, which are computed by averaging the flow field over time in the statistical steady state, that is,

$$\bar{\mathbf{u}}(\mathbf{x}) = \frac{1}{T}\int_{t_0}^{t_0+T} \mathbf{u}(\mathbf{x}, t)\,\mathrm{d}t, \tag{6}$$

where $t_0$ is the initial transient that ensures that the system is equilibrated, and $T$ is the sampling time.

## III. BASIC OBSERVATIONS

In this section, we report basic observations from our simulations of flow in rough channels, which may be useful for reproduction purposes.

### A. Effective aperture field

It is well known in the literature that the *actual* fracture width is not limited by the vertical width (along the $z$ coordinate), $d$, but rather by an *effective* channel width $d_{\mathrm{eff}}$, which can be better approximated as the smallest distance between the channel walls measured perpendicularly to the local flow direction [2, 17]. Since this direction changes along the rough surface, it consitutes an *effective aperture field* in the $xy$ plane. In our simulations, the vertical displacement is given by $d = 1$ everywhere, but the effective aperture depends sensitively and non-trivially on the roughness of the surfaces.

Now, we estimate the effective aperture field on purely geometrical grounds. The method we use is based on that by Mourzenko *et al.* [18], who suggested to fit the largest possible sphere at each point in the fracture to calculate the effective aperture. At a given in-plane coordinate $(x, y)$, we locate a sphere of radius $R(z)$ centered at $(x, y, z)$. Varying $z$, we seek a sphere of such a size that it barely touches the lower and upper channel walls, i.e. find the $z$ for which the minimal distance to the above surface equals the minimum distance to the lower surface. This gives us an optimum $z = z_{\mathrm{opt}}$ and a smallest effective channel width, $d_{\mathrm{eff}} = 2R(z_{\mathrm{opt}})$. Doing this for all $(x, y) \in [0, L] \times [0, L]$, we obtain the fields $z_{\mathrm{opt}}(x, y)$ (not shown) and $d_{\mathrm{eff}}(x, y)$. The former can be related to the tortuosity of the flow field [19]. The latter, which is of primary interest here, is a geometric approximation to the effective aperture field.

The effective aperture fields $d_{\mathrm{eff}}(x, y)$ are shown in Fig. 4 for increasing roughness. Here, it can be readily seen that the effective width depends strongly on the roughness amplitude, and for higher roughness, some areas are shielded by the most pronounced fracture tooths. In particular, it seems that an area with particularly low

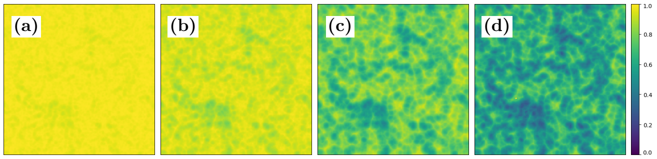


FIG. 4. Effective aperture field $d_{\rm eff}(x, y)$ for increasing roughness amplitude $A$. Subfigures (a)–(d) correspond to (b)–(e) in Fig. 2.

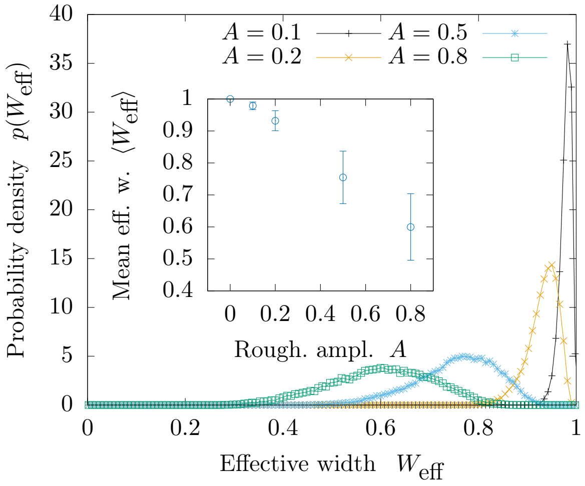


FIG. 5. Probability density of the effective aperture fields $d_{\rm eff}$ sampled over the plane $(x, y)$. Inset: The mean of the distributions in the main panel, with the standard deviations plotted as bars.

permeability emerges near the lower left corner, mimicking an obstacle.

It is also of interest to inspect the probability density functions of the effective aperture, sampled over the $xy$ plane, which are shown in Fig. 5. We note that the distributions are slightly skewed, decrease as the roughness amplitudes increases, and seem to approach a normal distribution for the highest roughness. This is further seen in the inset, where we show the dependence of the mean effective aperture upon the roughness amplitude.

### B. Qualitative inspection of the velocity fields

We now turn to inspecting the velocity fields that arise in the self-affine channels as a body force (or average pressure gradient) $\mathbf{f}$ is imposed.

To qualitatively visualize the spatial distribution of local fluxes, we consider depth-averaged velocity fields, i.e. the velocity fields in the $xy$ plane that result from averaging over $z \in [h, d + h]$. First, we present plots of the flow fields in the fully laminar, low inertia regime (Re $\sim 1$), shown in Fig. 6 for all velocity components normalized by $\langle u_x \rangle$. It is clear that similar features are present for all roughness amplitudes. In particular, one obstacle (the dark region in rows 1 and 2) leads to flow being directed around it. A bottleneck effect may result from this (see [20]), but this effect will be significantly smaller in 3D than in 2D fractures, since the flow is allowed to simply pass around the obstacle [2].

We present in Fig. 7 corresponding plots to the above, and show the depth-averaged time-averaged velocity fields $\bar{\mathbf{u}}$ for varying roughness. From these plots, in particular by inspecting $u_x$ (row 1), it is clear that at low roughness, preferential paths emerge that extend across the finite system. The slowest channel coincides with the obstacle noticed in the low Re regime (cf. Fig. 6). For higher roughness, this effect is less noticeable, in particular, the obstacle region cannot be seen for $u_x$ (but it is possible to see it for $u_y$). This is possibly because the roughness amplitude is so high that there is now no continuous straight chord that connects the flow field "to itself" (through the periodic boundary condition).


[1] E. Bouchaud, J. Phys. Condens. Matter **9**, 4319 (1997).
[2] E. Skjetne, A. Hansen, and J. Gudmundsson, J. Fluid Mech. **383**, 1 (1999).
[3] Y. Méheust and J. Schmittbuhl, Pure. Appl. Geophys. **160**, 1023 (2003).
[4] E. Bouchaud, G. Lapasset, and J. Planes, Europhys. Lett. **13**, 73 (1990).
[5] A.-L. Barabási and H. E. Stanley, *Fractal concepts in surface growth* (Cambridge University Press, 1995).
[6] R. F. Voss, in *Fundamental algorithms for computer graphics* (Springer, 1985) pp. 805–835.
[7] A. Klöckner, "Meshpy," `https://mathema.tician.de/software/meshpy/` (2018).
[8] J. R. Shewchuk, in *Applied Computational Geometry: Towards Geometric Engineering*, Lecture Notes in Computer Science, Vol. 1148, edited by M. C. Lin and D. Manocha (Springer-Verlag, 1996) pp. 203–222.
[9] H. Si, ACM Trans. Math. Softw. **41**, 11:1 (2015).
[10] M. Mortensen and K. Valen-Sendstad, Comput. Phys. Commun. **188**, 177 (2015).
[11] R. D. Moser, J. Kim, and N. N. Mansour, Phys. Fluids **11**, 943 (1999).
[12] A. Logg, K.-A. Mardal, and G. Wells, *Automated solution of differential equations by the finite element method: The FEniCS book*, Vol. 84 (Springer Science & Business Media, 2012).
[13] A. Logg, G. N. Wells, and J. Hake, in *Automated Solution of Differential Equations by the Finite Element Method* (Springer, 2012) pp. 173–225.
[14] S. Balay, S. Abhyankar, M. F. Adams, J. Brown, P. Brune, K. Buschelman, L. Dalcin, V. Eijkhout, W. D. Gropp, D. Kaushik, M. G. Knepley, D. A. May, L. C. McInnes, K. Rupp, B. F. Smith, S. Zampini, H. Zhang, and H. Zhang, "PETSc web page," `http://www.mcs.anl.gov/petsc` (2017).
[15] H. Jasak, A. Jemcov, Z. Tukovic, *et al.*, in *International*

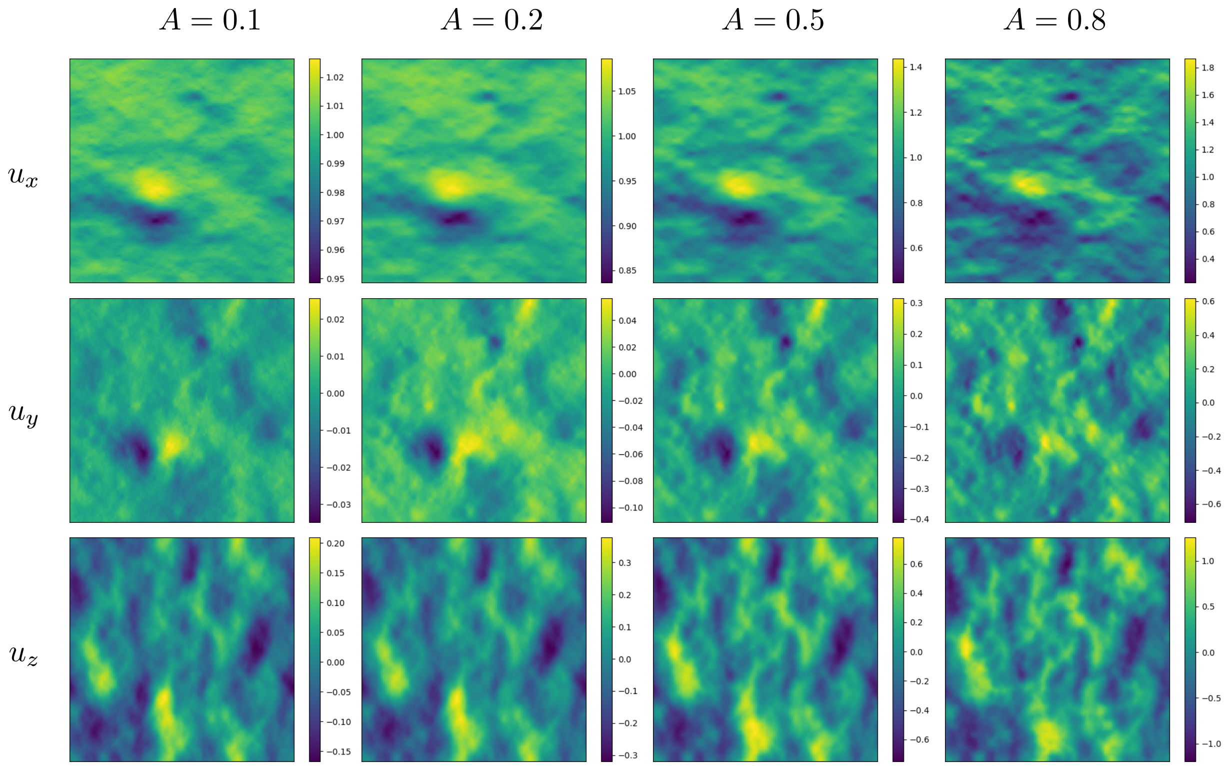


FIG. 6. Depth-averaged velocity fields for low Re, i.e. laminar flow. The figure shows the three components of the velocity vector, for four values of roughness amplitude $A$. The velocity components are normalized by $\langle u_x \rangle$.

*workshop on coupled methods in numerical dynamics*, Vol. 1000 (IUC Dubrovnik, Croatia, 2007) pp. 1–20.

[16] It is perhaps more common to define the Reynolds number, Re, based on the channel half-width and the maximum velocity of the equivalent laminar PPF flow profile (see [21, 22]), $\mathrm{Re}_h = u_{\max} W/(2\nu)$. There is no simple relation between the maximum and mean velocity in rough boundary flows, which makes Eq. (5) a more practical definition. In unidirectional PPF (laminar or turbulent), $\mathrm{Re}_h = \frac{3}{4}\mathrm{Re}$.

[17] B. Berkowitz, Adv. Water Resour. **25**, 861 (2002).

[18] V. V. Mourzenko, J.-F. Thovert, and P. M. Adler, J. Phys. II **5**, 465 (1995).

[19] A. Duda, Z. Koza, and M. Matyka, Phys. Rev. E **84**, 036319 (2011).

[20] L. Talon, H. Auradou, and A. Hansen, Water Resour. Res. **46**, W07601 (2010).

[21] X. Xiong, J. Tao, S. Chen, and L. Brandt, Phys. Fluids **27**, 041702 (2015).

[22] M. Sano and K. Tamai, Nat. Phys. **12**, 249 (2016).

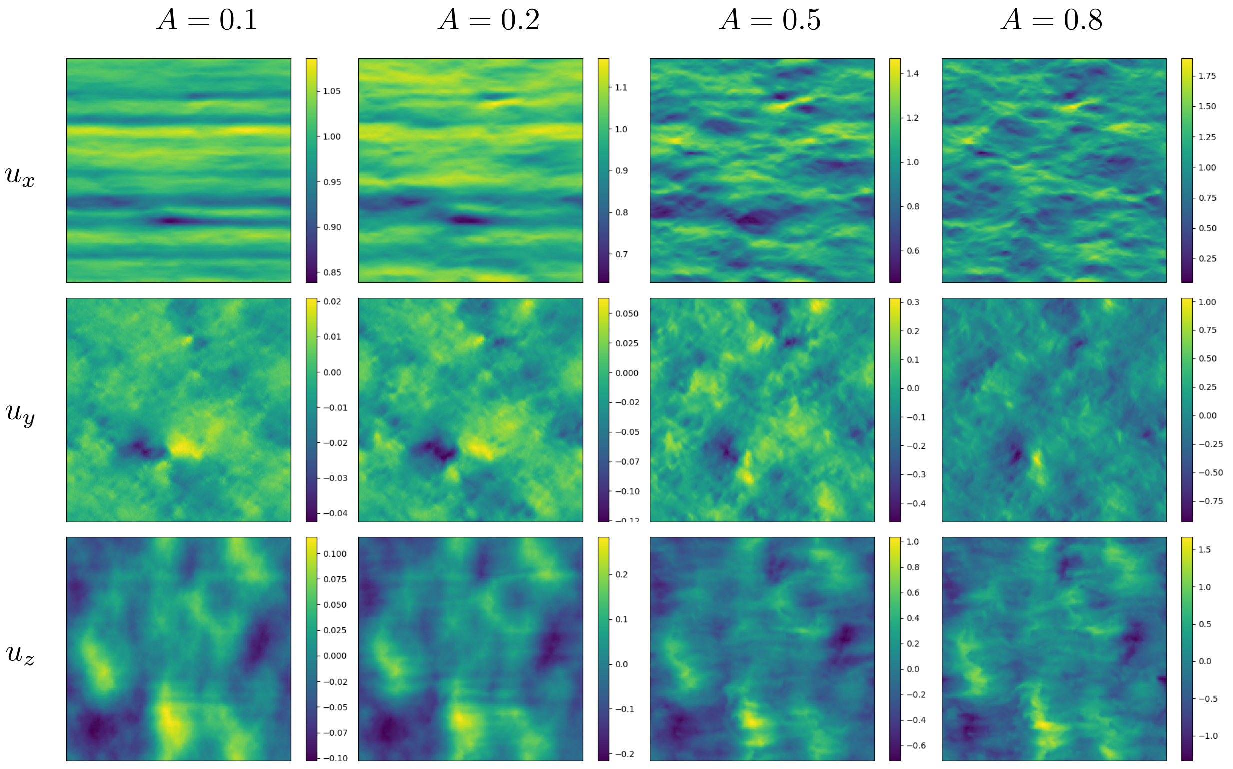


FIG. 7. The depth-and-time-averaged velocity field from high-Re simulations. Rows and columns correspond to Fig. 6.
